# Supplementary material for: Vision-based control of a knuckle boom crane with online cable length estimation
Source: arXiv:2005.11794 source file (2020-05-26)
Supplement: Supplementary file 1 [file 7Appendix.tex]

%\begin{algorithm}
%\caption{Extended Kalman Filter Implementation}
%\label{array-sum}
%\begin{algorithmic}[1]
%    \State $k=1$, $\hat{\bm{z}}_{k-1}=\bm{z}_0$, $\hat{\bm{P}}_{k-1}=\hat{\bm{P}}_0$
%    \Loop 
 %       \State $\bar{\bm{z}}_{k}=\bm{F}_d\hat{\bm{z}}_{k-1}+\bm{B}_d\bm{u}_{k-1}$
 %       \State $\bar{\bm{P}}_{k}=\bm{F}_d\hat{\bm{P}}_{k-1}\bm{F}_d^\tr+\bm{Q}$
 %       \State $\bm{K}_{k}=\bar{\bm{P}}_{k}\bm{H}_d^\tr\left(\bm{R}+\bm{H}\bar{\bm{P}}_{k}\bm{H}_d^\tr\right)^\inv$
 %       \State $\hat{\bm{z}}_{k}=\bar{\bm{z}}_{k}+\bm{K}_{k}\left(\bm{y}_{k}-\bm{H}_d\bar{\bm{z}}_{k}\right)$
 %       \State $\hat{\bm{P}}_{k}=\left(\bm{I}-\bm{K}_{k}\bm{H}_d\right)\bar{\bm{P}}_{k}\left(\bm{I}-\bm{K}_{k}\bm{H}_d\right)^\tr+\bm{K}_{k}\bm{R}\bm{K}_{k}^\tr$
 %       \State $k=k+1$
%	\EndLoop
%\end{algorithmic}
%\label{alg:euler}
%\end{algorithm}
